# Supplementary material for: XENONnT Analysis: Signal Reconstruction, Calibration and Event Selection
Source: arXiv:2409.08778 source file (2024-09-13)
Supplement: Supplementary file 1 [file appendix.tex]

\appendix

\section{Skewness -TO DO}
\label{sec:skew_gauss_ces}

The skew Gaussian model define as 

\begin{equation}
N e^{\frac{-(E-\xi)^2}{w^2}}\left(1+\operatorname{erf}\left(\alpha \frac{E-\xi}{w \sqrt{2}}\right)\right),
\end{equation}

where $\alpha$ is the skewness, $\xi$ and $w$ are two parameters that related to mean value and variance, but not exactly the same as them. The mean value of the skew Gaussian is given by:

\begin{equation}
\mu = \xi+\sqrt{\frac{2}{\pi}} \frac{\alpha w}{\sqrt{1+\alpha^2}}
\end{equation}

and the variance is given by:

\begin{equation}
\sigma = w^2\left(1-\frac{2}{\pi} \frac{\alpha^2}{1+\alpha^2}\right)
\end{equation}

\begin{equation}
\begin{aligned}
\frac{w}{E} & =\frac{a}{E}+b \\
a & =c \times E^{(d+1)}
\end{aligned}
\end{equation}

The fitted paranteters are $a = (37.2 \pm 0.4) \times 10^{-2}$\;keV, $b = (4.36 \pm 0.06) \times 10^{-3}$, $c = (1.999 \pm 0.006) \times 10^{-2}\;mathrm{keV}^{-(d+1)}$, and $d = (-1.256 \pm 0.002)$.

\section{Something Else if necessary}
